# Supplementary material for: Entropic anomaly and maximal efficiency of microscopic heat engines
Source: arXiv:1212.1608 source file (2012-12-07)
Supplement: Supplementary file 1 [file supp1.pdf]

# Entropic anomaly and the maximal efficiency of microscopic heat engines Supplementary Information

Stefano Bo[1,2] and Antonio Celani[3]

[1] *Cancer Cell Biophysics, IRC@C: Institute for Cancer Research at Candiolo, Str. Prov. 142 km 3.95, 10060 Candiolo, Torino, Italy*

[2] *INFN, via P. Giuria 1, 10125 Torino, Italy*

[3] *Physics of Biological Systems, Institut Pasteur and CNRS UMR 3525, 28 rue du docteur Roux, 75015 Paris, France*

(Dated: December 3, 2012)

## LANGEVIN-KRAMERS DYNAMICS

The general form of the Langevin-Kramers dynamics is given in Eq. (2) in the main text. In order to have a more concise notation we adopt its non-dimensional expression by introducing the following rescalings:

$$X \to \frac{X}{L} \qquad V \to V\sqrt{\frac{m}{k_B T_0}} \qquad f \to \frac{f}{k_B T_0/L}$$
$$T \to \frac{T}{T_0} \qquad t \to t\frac{\sqrt{k_B T_0/m}}{L} \qquad \gamma \to \frac{\gamma L}{\sqrt{k_B T_0 m}}$$

where $T_0$ is a reference temperature, $k_B$ the Boltzmann constant, $m$ the mass of the particle and $L$ the typical length scale of the process. This leads to

$$\begin{aligned} dX_t^i &= V_t^i dt \\ dV_t^i &= f^i(X_t,t)dt - \gamma(X_t,t)V_t^i dt + \sqrt{2T(X_t,t)\gamma(X_t,t)}\, dW_t^i \end{aligned} \tag{S1}$$

where $W_t^i$ are independent Wiener processes. Since trajectories are differentiable in space there is no ambiguity in the discretization procedure. In the following we shall abridge the notation by omitting the explicit dependency on the trajectory, e.g. $f^i(X_t,t) \equiv f_t^i$.

The associated Fokker-Planck (forward Kolmogorov) equation is

$$\frac{\partial p}{\partial t} + v^i \frac{\partial p}{\partial x^i} + f^i \frac{\partial p}{\partial v^i} - \gamma \frac{\partial}{\partial v^i}\left(v^i p\right) = T\gamma \frac{\partial^2 p}{\partial v^i \partial v^i} \tag{S2}$$

## STOCHASTIC THERMODYNAMICS

We provide here the definitions of the most relevant thermodynamic quantities following [1] and [2]. We consider temperature, friction and external forces to be smooth functions of space and time. The force $f^i$ may contain conservative and non-conservative contributions

$$f^i = -\frac{\partial U}{\partial x^i} + f^i_{nc} \,.$$

The energy of the particle is

$$E_t = U_t + \frac{V_t^i V_t^i}{2}$$

and the heat released into the environment

$$Q = \int_{t'}^{t} f_s^i \circ dX_s^i - V_s^i \circ dV_s^i \,.$$

where $\circ$ denotes the Stratonovich product.

The work performed on the particle is

$$W = \int_{t'}^{t} \frac{\partial U_s}{\partial s} ds + f^i_{nc,s} \circ dX_s^i = E_t - E_{t'} + Q \,.$$

It follows that energy is conserved along individual trajectories. This is the stochastic equivalent of the first principle of thermodynamics. Notice that the extracted work is simply defined as the opposite of the performed work: $W_{extr} = -W$.

The entropy of the particle is

$$S_p = -\log p(x, v, t)$$

where $p$ is the solution of (S2).

The entropy produced in the environment from an initial state $(X_{t'}, V_{t'})$ at time $t'$ to a final state $(X_t, V_t)$ at time $t$ is

$$S_{env} = \int_{t'}^{t} \frac{f_s^i}{T_s} \circ dX_s^i - \frac{V_s^i}{T_s} \circ dV_s^i \ . \tag{S3}$$

The total entropy change of particle and environment is

$$S_{tot} = -\log p_t + \log p_{t'} + \int_{t'}^{t} \frac{1}{T_s} \left( f_s^i \circ dX_s^i - V_s^i \circ dV_s^i \right) \ .$$

## Rate of heat release to a given thermostat

When the thermal environment is inhomogeneous it is necessary to separately consider the heat exchanges that take place at different temperatures. Let us consider the average entropy production during a cyclic process

$$\langle S_{tot} \rangle = \langle S_{env} \rangle = \left\langle \oint ds \frac{1}{T_s} \left( f_s^i \circ \dot{X}_s^i - V_s^i \circ \dot{V}_s^i \right) \right\rangle = -\oint ds \left\langle \gamma_s \frac{(nT_s - V_s^i V_s^i)}{T_s} \right\rangle \geq 0$$

where $T_s = T(X_s, s)$.

This can be rewritten as

$$\langle S_{tot} \rangle = \oint ds \int d\hat{T} \frac{1}{\hat{T}} \hat{p}(s, \hat{T}) \dot{q}(s, \hat{T})$$

where

$$\hat{p}(t, \hat{T}) d\hat{T} = \left\langle \delta \left( \hat{T} - T(X_t, t) \right) \right\rangle d\hat{T}$$

is the probability that the particle at time $t$ is in contact with the thermostat at temperature $(\hat{T}, \hat{T} + d\hat{T})$ and

$$\dot{q}(t, \hat{T}) = \left\langle \gamma_t \left( V_t^i V_t^i - nT_t \right) \middle| \hat{T} \right\rangle = \frac{\left\langle \left( f_t^i \circ \dot{X}_t^i - V_t^i \circ \dot{V}_t^i \right) \delta \left( \hat{T} - T_t \right) \right\rangle}{\left\langle \delta \left( \hat{T} - T_t \right) \right\rangle} = -\frac{\left\langle \gamma_t \left( nT_t - V_t^i V_t^i \right) \delta \left( \hat{T} - T_t \right) \right\rangle}{\left\langle \delta \left( \hat{T} - T_t \right) \right\rangle} \tag{S4}$$

is the average rate of heat release to the thermostat at temperature $\hat{T}$.

We are interested in deriving the asymptotic expressions for these quantities in the limit of vanishingly small inertia. This is done in two steps. In the next section we derive the limit for the propagator, i.e. the solution of the Fokker-Planck equation. Then, in the following section, the expression for $\dot{q}$.

## SMALL-INERTIA LIMIT

### *The propagator of the Fokker-Planck equation*

In this section we provide a derivation of the small-inertia (strong-friction) limit of the forward Kolmogorov equation (Fokker-Planck) [3]. The result defines the overdamped dynamics. Introducing the bookkeeping parameter $\epsilon$ and defining $\gamma = \epsilon^{-1}\tilde{\gamma}$, Eq. (S2) reads

$$\left( \frac{\partial}{\partial t} - L^\dagger - \epsilon^{-1} M^\dagger \right) p = 0$$

where

$$L_0 = v^i \frac{\partial}{\partial x^i} + f^i \frac{\partial}{\partial v^i} \qquad\qquad M = \tilde{\gamma}\left[-v^i \frac{\partial}{\partial v^i} + T \frac{\partial}{\partial v^i}\frac{\partial}{\partial v^i}\right]$$

The limit $\epsilon \to 0$ is a singular perturbation problem that can be treated by standard asymptotic methods.

As a first step one introduces a fast time variable $\theta = \epsilon^{-1} t$, associated to frictional relaxation, and a slow one $\tilde{t} = \epsilon t$. Force, temperature and friction are assumed to vary on the slow timescale only.

The propagator is assumed to be a function of fast, intermediate and slow times, and developed in power series in $\epsilon$ as $p = p^{(0)} + \epsilon p^{(1)} + \epsilon^2 p^{(2)} \ldots$.

*Fast time-scales.* Here we show that the dynamics at fast timescales (of the order of the inverse friction) is ruled by the balance of thermal noise and friction, and leads to relaxation to the Maxwell-Boltzmann distribution in velocity space, with the local temperature.

At order $\epsilon^{-1}$ the forward Kolmogorov equation reads

$$\left(\frac{\partial}{\partial \theta} - M^\dagger\right) p^{(0)} = 0$$

The eigenfunctions of $M^\dagger$ are products of Hermite polynomials in the velocity variable multiplied by the weight

$$w(v, x) = \frac{\exp\left(-\frac{v^2}{2T}\right)}{\left(2\pi T\right)^{n/2}}$$

i.e. the local Maxwell-Boltzmann equilibrium,

$$\psi_{k_1,\ldots,k_n} = w \prod_{i=1}^{n} H_{k_i}(v^i/\sqrt{T}) \qquad M\psi_{k_1,\ldots,k_n} = -\tilde{\gamma}\left(\sum_{i=1}^{n} k_i\right)\psi_{k_1,\ldots,k_n}$$

with $k_i = 0, 1, \ldots$. Since the spectrum is negative, the solution relaxes exponentially fast to the zero eigenfunction for $\theta \to \infty$

$$p^{(0)}(x, v, t, \tilde{t}) = \rho(x, t, \tilde{t}) w(x, v, \tilde{t})$$

where $\rho$ is the marginal probability density in space, at lowest order.

*Intermediate time-scales.* In this paragraph we show that at intermediate time-scales the system reaches an out-of equilibrium steady-state dictated by the balance of forces and temperature gradients. The dependence on the slow time-scale of variation of protocol, temperature and friction is still parametric.

At order $\epsilon^0$ one has

$$\left(\frac{\partial}{\partial \theta} - M^\dagger\right) p^{(1)} = -\left(\frac{\partial}{\partial t} - L_0^\dagger\right) p^{(0)}$$

which relaxes on fast timescales to the solution of

$$M^\dagger p^{(1)} = \left(\frac{\partial}{\partial t} - L_0^\dagger\right) p^{(0)}$$

The solvability condition for the previous equation requires that the r.h.s. be orthogonal to the null-space of $M$. In particular, it has to be orthogonal to all constants (functions that do not depend on $v$). Integrating the r.h.s. over $v$ all terms vanish by reflection symmetry but one

$$\frac{\partial \rho}{\partial t} = 0$$

This implies that the dependence on time for $\rho$ is only through slow timescales $\tilde{t}$, i.e. $p^{(0)}$ reaches a quasi-steady-state at intermediate time-scales where the dependence on slow time-scales enters as a parameter only.

Proceeding to solve the equation at order $\epsilon^0$ one has

$$M^\dagger p^{(1)} = -L_0^\dagger p^{(0)} = \left(v^i \frac{\partial}{\partial x^i} + f^i \frac{\partial}{\partial v^i}\right)(\rho w) = w v^i \frac{\partial \rho}{\partial x^i} + \rho v^i \frac{\partial w}{\partial x^i} + \rho f^i \frac{\partial w}{\partial v^i}$$

$$= wv^i \frac{\partial \rho}{\partial x^i} + \rho w v^i \frac{\left(v^j v^j - nT\right)}{2T^2} \frac{\partial T}{\partial x^i} - \rho \frac{f^i v^i}{T} w$$

Noticing that

$$M^\dagger \left(v^i w\right) = -\tilde{\gamma} v^i w \qquad M^\dagger \left[\left((n+2)Tv^i - v^i v^j v^j\right) w\right] = -3\tilde{\gamma}\left((n+2)Tv^i - v^i v^j v^j\right) w$$

one obtains

$$p^{(1)} = rw - \frac{v^i}{\tilde{\gamma}} \frac{\partial \rho}{\partial x^i} w + \frac{v^i}{\tilde{\gamma} T} \left(f^i - \frac{\partial T}{\partial x^i}\right) \rho w + \frac{\left((n+2)T - v^j v^j\right) v^i}{6\tilde{\gamma} T^2} \frac{\partial T}{\partial x^i} \rho w$$

where $r = r(x, \tilde{t})$ and $rw$ is the contribution from the null-space of $M^\dagger$.

*Slow time-scales.* At these scales we obtain the overdamped dynamics.

At order $\epsilon^1$ one has, after relaxation over fast variables,

$$M^\dagger p^{(2)} = -L_0^\dagger p^{(1)} + \frac{\partial}{\partial \tilde{t}} p^{(0)} \tag{S5}$$

The solvability condition is again obtained by integrating both sides over $v$. Notice that the integrals of the first and the last term from $p^{(1)}$ vanish and thus do not contribute to the spatial flux of probability. It follows that

$$\frac{\partial \rho}{\partial \tilde{t}} + \frac{\partial}{\partial x^i} \left(\frac{f^i}{\tilde{\gamma}} \rho\right) = \frac{\partial}{\partial x^i} \frac{1}{\tilde{\gamma}} \frac{\partial}{\partial x^i} T\rho$$

Reverting to the original time-scales $t = \epsilon^{-1}\tilde{t}$ and friction $\gamma = \epsilon^{-1}\tilde{\gamma}$ one therefore obtains

$$\frac{\partial \rho}{\partial t} + \frac{\partial}{\partial x^i} \left(\frac{f^i}{\gamma} \rho\right) = \frac{\partial}{\partial x^i} \frac{1}{\gamma} \frac{\partial}{\partial x^i} T\rho \, .$$

The limiting (overdamped) process is therefore generated by

$$\mathcal{L} = \frac{f^i}{\gamma} \frac{\partial}{\partial x^i} + T \frac{\partial}{\partial x^i} \frac{1}{\gamma} \frac{\partial}{\partial x^i}$$

which corresponds to the following SDE:

$$dX_t^i = \left(\frac{f^i}{\gamma} - \frac{1}{2\gamma} \frac{\partial T}{\partial x^i} + \frac{T}{2} \frac{\partial \gamma^{-1}}{\partial x^i}\right) dt + \sqrt{\frac{2T}{\gamma}} \circ dw_t^i \tag{S6}$$

where the $\circ$ indicates that the product is taken with the Stratonovich midpoint convention. The Itô non-anticipative product will be denoted by the $\cdot$ symbol:

$$dX_t^i = \left(\frac{f^i}{\gamma} + T \frac{\partial \gamma^{-1}}{\partial x^i}\right) dt + \sqrt{\frac{2T}{\gamma}} \cdot dw_t^i \tag{S7}$$

Notice that in the main text all products are meant in the Stratonovich sense.

### *Small inertia limit of the rate of heat release to a given thermostat*

We now derive the limiting behavior of the rate of heat release to a given thermostat in presence of vanishing inertia. Making use of the expansion for the probability density derived in the previous section we can express the functional (S4) as

$$\hat{p}(t, \hat{T}) \dot{q}(t, \hat{T}) = -\epsilon^{-1} \int d\boldsymbol{x} d\boldsymbol{v} \; \delta(T(x,t) - \hat{T}) \tilde{\gamma} \left(nT - v^i v^i\right) \left(p^{(0)} + \epsilon p^{(1)} + \epsilon^2 p^{(2)} + \dots\right) \, .$$

Since the contributions at orders $\epsilon^0$ and $\epsilon$ do not project on the second-order Hermite polynomial one has

$$\hat{p}(t, \hat{T}) \dot{q}(t, \hat{T}) = -\epsilon \int d\boldsymbol{x} \; \delta(T(x,t) - \hat{T}) \tilde{\gamma} \int d\boldsymbol{v} \; \left(nT - v^i v^i\right) p^{(2)} + \dots$$

The latter integral can be evaluated by projecting the equation for $p^{(2)}$ on the Hermite polynomial

$$\int d\boldsymbol{v}\ \left(nT - v^i v^i\right) M^\dagger p^{(2)} = -2\int d\boldsymbol{v}\ \tilde{\gamma}\left(nT - v^i v^i\right) p^{(2)} = \int d\boldsymbol{v}\ \left(nT - v^i v^i\right)\left(-L_0^\dagger p^{(1)} + \frac{\partial}{\partial \tilde{t}} p^{(0)}\right)$$

where the first term is equal to the last one according to equation (S5). Now noticing that

$$\frac{\partial}{\partial \tilde{t}} p^{(0)} = \frac{\partial \rho}{\partial \tilde{t}} w + \frac{\partial \log w}{\partial \tilde{t}} \rho w = \frac{\partial \rho}{\partial \tilde{t}} w - \frac{1}{2T^2}\frac{\partial T}{\partial \tilde{t}}\left(nT - v^i v^i\right)\rho w$$

and

$$\left(nT - v^j v^j\right)(-L_0^\dagger) p^{(1)} = \left(nT - v^j v^j\right)\left(v^i \frac{\partial}{\partial x^i} + f^i \frac{\partial}{\partial v^i}\right) p^{(1)} =$$

$$= \frac{\partial}{\partial x^i}\left[\left(nT - v^j v^j\right) v^i p^{(1)}\right] - n\frac{\partial T}{\partial x^i} v^i p^{(1)} + \frac{\partial}{\partial v^i}\left[\left(nT - v^j v^j\right) f^i p^{(1)}\right] + 2 v^i f^i p^{(1)}$$

$$= \frac{\partial}{\partial x^i}\left[\left((n+2)T - v^j v^j\right) v^i p^{(1)}\right] - n\frac{\partial T}{\partial x^i} v^i p^{(1)} + \frac{\partial}{\partial v^i}\left[\left(nT - v^j v^j\right) f^i p^{(1)}\right] + 2 v^i f^i p^{(1)} - 2\frac{\partial}{\partial x^i}\left(T v^i p^{(1)}\right)$$

the integration over velocity gives

$$\int d\boldsymbol{v}\ \left((n+2)T - v^j v^j\right) v^i p^{(1)} = \frac{(n+2)}{3\tilde{\gamma}} T \frac{\partial T}{\partial x^i}\rho$$

$$\int d\boldsymbol{v}\ v^i p^{(1)} = -\frac{T}{\tilde{\gamma}}\frac{\partial \rho}{\partial x^i} + \frac{1}{\tilde{\gamma}}\left(f^i - \frac{\partial T}{\partial x^i}\right)\rho\ .$$

These combine to give

$$\int d\boldsymbol{v}\ \left(nT - v^i v^i\right)\left(-L_0^\dagger p^{(1)} + \frac{\partial}{\partial \tilde{t}} p^{(0)}\right) =$$

$$\frac{\partial}{\partial x^i}\left[\frac{(n+2)}{3\tilde{\gamma}} T \frac{\partial T}{\partial x^i}\rho\right] + 2\left(f^i - \frac{n}{2}\frac{\partial T}{\partial x^i}\right)\left[-\frac{T}{\tilde{\gamma}}\frac{\partial \rho}{\partial x^i} + \frac{1}{\tilde{\gamma}}\left(f^i - \frac{\partial T}{\partial x^i}\right)\rho\right] - 2\frac{\partial}{\partial x^i}\left[-\frac{T^2}{\tilde{\gamma}}\frac{\partial \rho}{\partial x^i} + \frac{T}{\tilde{\gamma}}\left(f^i - \frac{\partial T}{\partial x^i}\right)\rho\right] - n\frac{\partial T}{\partial \tilde{t}}\rho$$

from which it follows that in the limit of vanishing inertia

$$\hat{p}(t,\hat{T})\dot{q}(t,\hat{T}) = \int d\boldsymbol{x}\ \delta\left(T(x,t) - \hat{T}\right)\left[\underbrace{\frac{\partial}{\partial x^i}\left(\frac{(n+2)}{6\gamma} T \frac{\partial T}{\partial x^i}\rho\right)}_{anom} + \underbrace{f^i J_i}_{ext} - \underbrace{\frac{\partial}{\partial x^i}\left(T J_i\right)}_{tp} - \underbrace{\frac{n}{2}\frac{\partial T}{\partial t}\rho - \frac{n}{2}\frac{\partial T}{\partial x^i} J_i}_{kin}\right]$$

where

$$J_i = -\frac{T}{\gamma}\frac{\partial \rho}{\partial x^i} + \frac{1}{\gamma}\left(f^i - \frac{\partial T}{\partial x^i}\right)\rho$$

is the probability flux. Making use of the identity

$$\int d\boldsymbol{x}\, \varphi^i J^i = \left\langle \varphi^i \circ \frac{dX^i}{dt}\right\rangle\ ,$$

integrating by parts and exploiting the properties of the delta function we can write the equation for the rate of heat release at given thermostat as:

$$\dot{q}(t,\hat{T}) = \underbrace{\hat{p}^{-1}\frac{\partial}{\partial \hat{T}}\left[\hat{p}\hat{T}\left\langle \frac{(n+2)}{6\gamma}\frac{\partial T}{\partial x^i}\frac{\partial T}{\partial x^i}\right\rangle_{T=\hat{T}}\right]}_{\dot{q}_{anom}} + \underbrace{\left\langle f_t^i \dot{X}_t^i\right\rangle_{T=\hat{T}}}_{\dot{q}_{ext}} \underbrace{-\hat{p}^{-1}\frac{\partial}{\partial \hat{T}}\left[\hat{p}\hat{T}\left\langle \frac{\partial T}{\partial x^i}\dot{X}_t^i\right\rangle_{T=\hat{T}}\right]}_{\dot{q}_{tp}} \underbrace{-\frac{n}{2}\left\langle \frac{dT}{dt}\right\rangle_{T=\hat{T}}}_{\dot{q}_{kin}} \qquad \text{(S8)}$$

where the averages are taken along overdamped trajectories.

It is useful to check that the current findings are consistent with those derived for entropy production in [3]. The average entropy production is

$$\langle S_{env}\rangle = -\int_{t'}^{t} ds \int d\boldsymbol{x}\frac{1}{T}\int d\boldsymbol{v}\,\gamma\left(nT - v^i v^i\right)p^{(2)} = \int_{t'}^{t} ds\int d\hat{T}\frac{1}{T}\hat{p}(s,\hat{T})\dot{q}(s,\hat{T}) =$$

$$\int_{t'}^{t} ds \int d\boldsymbol{x}\frac{1}{T}\left\{\underbrace{\frac{\partial}{\partial x^i}\left[\frac{(n+2)}{6\gamma}T\frac{\partial T}{\partial x^i}\rho\right]} + \left(f^i - \frac{n}{2}\frac{\partial T}{\partial x^i}\right)\left[-\frac{T}{\gamma}\frac{\partial \rho}{\partial x^i} + \frac{1}{\gamma}\left(f^i - \frac{\partial T}{\partial x^i}\right)\rho\right]\right.$$

$$\left. -\frac{\partial}{\partial x^i}\left[-\frac{T^2}{\gamma}\frac{\partial\rho}{\partial x^i} + \frac{T}{\gamma}\left(f^i - \frac{\partial T}{\partial x^i}\right)\rho\right] - \frac{n}{2}\frac{\partial T}{\partial t}\rho\right\}$$

$$= \int_{t'}^{t}\left\langle\frac{(n+2)}{6\gamma T}\frac{\partial T}{\partial x^i}\frac{\partial T}{\partial x^i}d\tau\right\rangle_{anom} + \left\langle\frac{1}{T}\left(f^i - \frac{\partial T}{\partial x^i}\right)\circ dx^i\right\rangle_{over} - \left\langle\frac{n}{2}d\log T\right\rangle_{kin}.$$

The first term is the anomaly, the second one is the regular entropy production, the third one cancels with the particle entropy, as expected.

To conclude this section we recover the usual expression for the net heat released by integrating over the different temperatures:

$$\langle Q\rangle = \int_{t'}^{t} ds\int d\boldsymbol{x}\int d\boldsymbol{v}\,\gamma\left(nT - v^i v^i\right)p^{(2)} = \int_{t'}^{t} ds\int d\hat{T}\hat{p}(s,\hat{T})\dot{q}(s,\hat{T}) =$$

$$\int_{t'}^{t} ds\int d\boldsymbol{x}\left\{\frac{\partial}{\partial x^i}\left[\frac{(n+2)}{6\gamma}T\frac{\partial T}{\partial x^i}\rho\right] + \left(f^i - \frac{n}{2}\frac{\partial T}{\partial x^i}\right)\left[-\frac{T}{\gamma}\frac{\partial\rho}{\partial x^i} + \frac{1}{\gamma}\left(f^i - \frac{\partial T}{\partial x^i}\right)\rho\right]\right.$$

$$\left. -\frac{\partial}{\partial x^i}\left[-\frac{T^2}{\gamma}\frac{\partial\rho}{\partial x^i} + \frac{T}{\gamma}\left(f^i - \frac{\partial T}{\partial x^i}\right)\rho\right] - \frac{n}{2}\frac{\partial T}{\partial t}\rho\right\}$$

$$= \int_{t'}^{t}\langle f^i \circ dx^i\rangle - \left\langle\frac{n}{2}dT\right\rangle$$

as expected. Notice that the divergence terms that were responsible for the anomalous and the thermophoretic entropic contributions here vanish (with natural boundary conditions on $\rho$). The associated divergence terms therefore do not provide a net heat exchange with the thermostats, only an internal transfer from hotter to colder thermostats, thereby producing entropy with/without an associated mass flux (thermophoretic/anomalous).

## STOCHASTIC CYCLIC HEAT ENGINES

### From entropy production to efficiency

The efficiency of a stochastic heat engine is defined as the ratio of the average extracted work to the average absorbed heat :

$$\eta = \frac{\langle W_{extr}\rangle}{\langle Q_{abs}\rangle} = 1 - \frac{\langle Q_{rel}\rangle}{\langle Q_{abs}\rangle} \tag{S9}$$

where

$$\langle Q_{rel}\rangle = \int d\hat{T} \oint dt\, \hat{p}\dot{q}\, \theta(\dot{q}) \geq 0 \qquad \langle Q_{abs}\rangle = -\int d\hat{T} \oint dt\, \hat{p}\dot{q}\, \theta(-\dot{q}) \geq 0$$

and of course $\langle Q\rangle = \langle Q_{rel}\rangle - \langle Q_{abs}\rangle$.

It is interesting to compare these definitions of absorbed and released heat with the expressions irrespective of the thermostat. Using Jensen's inequality $\langle z\theta(z)\rangle \geq \langle z\rangle\theta(\langle z\rangle)$ – where the averages are over the distributions of $\hat{T}$ – one can show that

$$\langle Q_{rel}\rangle \geq \oint dt\, \langle\dot{Q}\rangle\, \theta\left(\langle\dot{Q}\rangle\right) \qquad\qquad \langle Q_{abs}\rangle \geq \oint dt\, (-\langle\dot{Q}\rangle)\, \theta\left(-\langle\dot{Q}\rangle\right)$$

where

$$\langle\dot{Q}\rangle = \int d\hat{T}\hat{p}(t,\hat{T})\dot{q}(t,\hat{T})$$

is the net average rate of heat release.

The r.h.s. in the latter inequalities are the classical definitions of released and absorbed heat irrespective of the thermostat and are shown to be always less than or equal to the ones considering each thermostat. The equality occurs only if the distribution of $\hat{T}$ at any given time has support on a single value, i.e. in the homogeneous case. The inequality for $Q_{abs}$ implies, for $\langle W_{extr}\rangle > 0$,

$$\eta \leq -\frac{\langle W_{extr}\rangle}{\oint dt\, (-\langle\dot{Q}\rangle)\, \theta\left(-\langle\dot{Q}\rangle\right)} \equiv \eta_{uniform}$$

where $\eta_{uniform}$ is the efficiency defined by the overall heat exchange, summed over all reservoirs. In order to highlight the difference in efficiency between a homogeneous engine and a non-homogeneous one it is useful to express it in terms of entropy production. Also the entropy released in the environment (which for a cycle coincides with the total entropy production) can be split into a released term and an absorbed one as

$$\langle S_{env}\rangle = \langle S_{rel}\rangle - \langle S_{abs}\rangle = \frac{\langle S_{rel}\rangle}{\langle Q_{rel}\rangle}\langle Q_{rel}\rangle - \frac{\langle S_{abs}\rangle}{\langle Q_{abs}\rangle}\langle Q_{abs}\rangle = \frac{\langle Q_{rel}\rangle}{T_{rel}} - \frac{\langle Q_{abs}\rangle}{T_{abs}}$$

where $T_{rel}$ and $T_{abs}$ are the average temperatures weighted by entropy release and absorption rates over the cycle

$$T_{rel} = \frac{\int d\hat{T} \oint dt\, \hat{T}\dot{S}_{rel}}{\int d\hat{T} \oint dt\, \dot{S}_{rel}} = \frac{\langle Q_{rel}\rangle}{\int d\hat{T} \oint dt\, \dot{S}_{rel}} \qquad\qquad \dot{S}_{rel} = \frac{1}{\hat{T}}\hat{p}\dot{q}\theta(\dot{q}) \geq 0$$

$$T_{abs} = \frac{\int d\hat{T} \oint dt\, \hat{T}\dot{S}_{abs}}{\int d\hat{T} \oint dt\, \dot{S}_{abs}} = \frac{\langle Q_{abs}\rangle}{\int d\hat{T} \oint dt\, \dot{S}_{abs}} \qquad\qquad \dot{S}_{abs} = -\frac{1}{\hat{T}}\hat{p}\dot{q}\theta(-\dot{q}) \geq 0\ .$$

The above identity implies for the efficiency

$$\eta = \frac{1 - \frac{T_{rel}}{T_{abs}}}{1 + \frac{T_{rel}\langle S_{env}\rangle}{\langle W_{extr}\rangle}} \tag{S10}$$

which is equation (4) in the main text. In the absence of temperature gradients and in the quasi-equilibrium limit $\tau \to \infty$ and $\langle S_{tot}\rangle \to 0$

$$\eta \to 1 - \frac{T_{rel}^{\infty}}{T_{abs}^{\infty}} \qquad \text{(quasi-equilibrium, uniform temperature)}\ .$$

Conversely, in presence of gradients the anomalous entropy production dominates the denominator and one has

$$\eta \to \frac{\langle W_{extr}^{\infty}\rangle}{T_{rel}^{\infty}\langle S_{anom}\rangle}\left(1 - \frac{T_{rel}^{\infty}}{T_{abs}^{\infty}}\right) \sim \frac{\tilde{\tau}}{\tau} \qquad \text{(quasi-equilibrium with temperature gradient)}\ . \tag{S11}$$

Notice that the quasi-equilibrium temperatures $T_{rel/abs}^{\infty}$ in the presence of gradients are in general different from the ones in uniform temperature.

**A cyclic stochastic engine attaining Carnot efficiency**

Hereafter, friction is assumed constant, the nonconservative force is absent $f_{nc} = 0$ and we drop the explicit notation for the average over trajectories and therefore thermodynamic quantities, unless otherwise stated, are to be interpreted as average ones.

*Adiabatic transformations*

We consider the one dimensional case of a parabolic trap with variable stiffness exerting a linear force on a Brownian particle resulting in the SDE:

$$dX_t = \left(-k(t)\frac{X_t}{\gamma} - \frac{1}{2\gamma}\frac{\partial T}{\partial x}\right) dt + \sqrt{\frac{2T}{\gamma}} \circ dw_t \ .$$

A crucial ingredient in the construction of an engine capable of attaining Carnot efficiency is the definition of an adiabatic transformation. In a generic non-uniform environment this requires the vanishing of $\dot{q}(\hat{T})$ for all thermostats $\hat{T}$. This in turn implies the vanishing of entropy production, as it can also be seen by means of the bound on efficiency previously derived. Clearly, in presence of a temperature gradient, Carnot efficiency cannot be obtained because of the anomalous entropy production. Actually, no truly adiabatic transformation exists due to the corresponding anomalous term in the heat release that cannot be forced to vanish. However, Carnot efficiency can be approached for arbitrarily small gradients provided that the overdamped contribution to entropy production vanishes as well. This requires the system to be at quasi-equilibrium.

Given these considerations, we construct adiabatic transformations for a one-dimensional harmonic trap as follows. In absence of a temperature gradient, at a given time, all heat exchanges take place with the same thermostat and the average rate of heat release is

$$\dot{Q} = \left(-\frac{k}{2}\frac{d\sigma^2}{dt} - \frac{1}{2}\frac{dT_0}{dt}\right)$$

where the second term is the kinetic heat leakage. This equation goes along with the equation for the variance

$$\frac{d\sigma^2}{dt} = -2\frac{k}{\gamma}\sigma^2 + 2\frac{T_0}{\gamma}$$

where the average $\langle x \rangle$ is assumed to have already relaxed to zero. In the quasi-equilibrium limit

$$\sigma^2 \simeq \frac{T_0}{k} + O\left(\frac{\gamma}{k\tau}\right)$$

which gives

$$\dot{Q} = -\frac{dT_0}{dt} + \frac{T_0}{2k}\frac{dk}{dt} + o\left(\frac{\gamma}{k\tau}\right) = -\frac{k}{2T_0}\frac{d}{dt}\left(\frac{T_0^2}{k}\right) + o\left(\frac{\gamma}{k\tau}\right) \ .$$

This result suggests that the sought adiabatic transformation is given by the protocol

$$\frac{T_0^2}{k} = \text{constant} \qquad\qquad \text{(adiabatic)} \ .$$

The prefix pseudo serves to recall that during such transformations the heat exchange vanishes only in the quasi-equilibrium limit and in a thermally uniform environment.

*Carnot cycle*

Let us consider the following cyclic protocol

| | | |
|---|---|---|
| isothermal expansion | $T = T_h \qquad k = k_{max} + \frac{(k_{min} - k_{max})}{\tau_1} t$ | $0 \leq t \leq \tau_1$ |
| adiabatic expansion | $T = T_h + \frac{(T_c - T_h)}{\tau_2}(t - \tau_1) \qquad k = \frac{k_{min}}{T_h^2} T^2$ | $\tau_1 \leq t \leq \tau_1 + \tau_2$ |
| isothermal compression | $T = T_c \qquad k = \left[k_{min} + \frac{(k_{max} - k_{min})}{\tau_1}(t - \tau_1 - \tau_2)\right]\left(\frac{T_c}{T_h}\right)^2$ | $\tau_1 + \tau_2 \leq t \leq 2\tau_1 + \tau_2$ |
| adiabatic compression | $T = T_c + \frac{(T_h - T_c)}{\tau_2}(t - 2\tau_1 - \tau_2) \qquad k = \frac{k_{max}}{T_h^2} T^2$ | $2\tau_1 + \tau_2 \leq t \leq 2\tau_1 + 2\tau_2$ |

where $2\tau_1 + 2\tau_2 = \tau$.

In the quasi-equilibrium limit heat is absorbed during isothermal expansion and released during isothermal compression. No heat transfer takes place during adiabatic transformations. The total absorbed heat during the cycle is

$$Q_{abs}^{\infty} = -\int_0^{\tau_1} \dot{Q} dt = \frac{T_h}{2} \int_0^{\tau_1} k \frac{d}{dt}\left(\frac{1}{k}\right) dt = \frac{T_h}{2} \log\left(\frac{k_{max}}{k_{min}}\right) .$$

As for the extracted work

$$W_{extr}^{\infty} = -\frac{1}{2} \oint \dot{k} \sigma^2 dt = -\frac{1}{2} \oint \dot{k} \frac{T}{k} dt$$

$$= -\frac{1}{2}\left[-T_h \log\left(\frac{k_{max}}{k_{min}}\right) + (T_c - T_h) + T_c \log\left(\frac{k_{max}}{k_{min}}\right) + (T_h - T_c)\right] = \frac{1}{2}(T_h - T_c)\log\left(\frac{k_{max}}{k_{min}}\right) .$$

The ensuing asymptotic efficiency is Carnot

$$\eta^{\infty} = \frac{W_{extr}^{\infty}}{Q_{abs}^{\infty}} = 1 - \frac{T_c}{T_h} .$$

Remark that the quasi-equilibrium efficiency does not depend on the details of the protocol provided that is consists of two isothermal and two adiabatic transformations at quasi-equilibrium.

**Small gradient expansion**

In order to gain insight on cycles taking place in non-homogeneous environments we consider the (physically relevant) case of small temperature gradients *i.e.* gradients that result in small temperature differences on the typical length scales of the process:

$$T(\boldsymbol{x}, t) = T_0(t) + g^j x^j \qquad \frac{g\sigma}{T_0} \ll 1$$

where $\sigma = \langle x^j x^j \rangle^{1/2}$ is the standard deviation of the particle position. We discuss the $n-$dimensional case described by

$$dX_t^i = \left(-k(t)\frac{X_t^i}{\gamma} - \frac{1}{2\gamma} g^i\right) dt + \sqrt{\frac{2T}{\gamma}} \circ dw_t^i .$$

We start by deriving the solution of the Fokker-Planck equation for a harmonic trap in a linear gradient of temperature

$$\frac{\partial \rho}{\partial t} = \frac{\partial}{\partial x^i}\left(\frac{k(t)}{\gamma} x^i \rho\right) + \frac{\partial^2}{\partial x^i \partial x^i}\left(\frac{T_0(t) + g^j x^j}{\gamma}\rho\right) = \left(\mathcal{L}_0^{\dagger} + g^j \mathcal{M}_j^{\dagger}\right)\rho$$

in the limit of small gradients.

One seeks an expansion of the solution in a Hermite basis

$$\rho = \sum_{(l)} a_{(l)}(t)\psi_{(l)}(x,t)$$

where $(l) = (l_1, \dots, l_n)$ are nonnegative integers, and

$$\psi_{(l)}(x) = \prod_{i=1}^{n} \psi_{l_i}(x_i) \qquad \psi_{l_i}(z) = H_{l_i}\left(\frac{z}{\sigma}\right) \frac{e^{-\frac{z^2}{2\sigma^2}}}{(2\pi\sigma^2)^{1/2}} \ .$$

Above, $\sigma$ is the standard deviation of the distribution and evolves according to

$$\dot{\sigma} = -\frac{k}{\gamma}\sigma + \frac{T_0}{\gamma\sigma} \ .$$

The above functions have the noticeable properties

$$\frac{\partial^2}{\partial z^2}\psi_l = \frac{1}{\sigma^2}\psi_{l+2}$$

$$\left(\frac{\partial}{\partial z} z + \sigma^2 \frac{\partial^2}{\partial z^2}\right)\psi_l = -l\psi_l$$

$$\frac{\partial}{\partial t}\psi_l = \frac{\dot{\sigma}}{\sigma}\left(\psi_{l+2} + l\psi_l\right) \ .$$

One therefore has

$$\frac{\partial \psi_{(l)}}{\partial t} = \frac{\dot{\sigma}}{\sigma}\sum_{i=1}^{n}\left(\psi_{l_i+2} + l_i\psi_{l_i}\right)\prod_{j\neq i}\psi_{l_j} = \frac{\dot{\sigma}}{\sigma}\sum_{i=1}^{n}\left(\psi_{(l_1,\dots,l_i+2,\dots,l_n)} + l_i\psi_{(l_1,\dots,l_i,\dots,l_n)}\right)$$

and

$$\mathcal{L}_0^\dagger\psi_{(l)} = \frac{k}{\gamma}\sum_{i=1}^{n}\left[\left(\frac{\partial}{\partial x^i}x^i + \frac{T_0}{k}\frac{\partial^2}{\partial x^i \partial x^i}\right)\psi_{l_i}(x_i)\right]\prod_{j\neq i}\psi_{l_j}(x_j) = \frac{k}{\gamma}\sum_{i=1}^{n}\left[-l_i\psi_{(l_1,\dots,l_i,\dots,l_n)} + \left(\frac{T_0}{k\sigma^2} - 1\right)\psi_{(l_1,\dots,l_i+2,\dots,l_n)}\right]$$

from which it follows, using the equation for $\sigma$, that

$$\left(\frac{\partial}{\partial t} - \mathcal{L}_0^\dagger\right)\psi_{(l)} = \frac{T_0}{\gamma\sigma^2}\left(\sum_i l_i\right)\psi_{(l)}$$

i.e. $\partial/\partial t - \mathcal{L}_0^\dagger$ is diagonal in the chosen Hermite basis.

At first order in the gradient, the density obeys

$$\rho = \rho_0 + \rho_1 \qquad \left(\frac{\partial}{\partial t} - \mathcal{L}_0^\dagger\right)\rho_0 = 0 \qquad \left(\frac{\partial}{\partial t} - \mathcal{L}_0^\dagger\right)\rho_1 = g^j \mathcal{M}_j^\dagger \rho_0 \ .$$

Expanding in the diagonal basis one sees that the zero-th order term converges exponentially to the Gaussian solution

$$\rho_0 \to \psi_{(0)} = \frac{e^{-\frac{x^i x^i}{2\sigma^2}}}{(2\pi\sigma^2)^{n/2}} \ .$$

Then,

$$\sum_j g^j \mathcal{M}_j^\dagger \rho_0 = \frac{1}{\gamma}\sum_j 2g^j\frac{\partial\rho_0}{\partial x^j} + \sum_{i,j} g^j x^j \frac{\partial^2\rho_0}{\partial x^i \partial x^i} = \frac{1}{\gamma\sigma}\left[\sum_{i,j}\frac{g^j x^j x^i x^i}{\sigma^3} - (n+2)\frac{g^j x^j}{\sigma}\right]\rho_0$$

$$= \frac{1}{\gamma}\left[\sum_j \frac{g^j}{\sigma}\left(H_3\left(\frac{x_j}{\sigma}\right) + H_1\left(\frac{x_j}{\sigma}\right)\sum_{i\neq j} H_2\left(\frac{x_i}{\sigma}\right)\right)\right]\rho_0 \ .$$

Choosing the direction of the gradient along the $x_1$ axis for the sake of simplicity, the above formula can be rewritten in terms of basis functions as

$$\sum_j g^j \mathcal{M}_j^\dagger \rho_0 = \frac{g}{\sigma}\left(\psi_{(3,0,\dots,0)} + \sum_{i=2}^{n} \psi_{(1,0,\dots,\underbrace{2}_{i-\mathrm{th}},\dots,0)}\right) \ .$$

It follows immediately that the first-order term in the density is

$$\rho_1 = \frac{g\sigma}{3T_0}\left(\psi_{(3,0,\dots,0)} + \sum_{i=2}^{n} \psi_{(1,0,\dots,\underbrace{2}_{i-\mathrm{th}},\dots,0)}\right) \ .$$

In one dimension the solution for small gradients of the Fokker-Planck equation is therefore

$$\rho = \left[1 + \frac{g\sigma}{3T_0}\left(\frac{x^3}{\sigma^3} - 3\frac{x}{\sigma}\right)\right]\frac{e^{-\frac{x^2}{2\sigma^2}}}{\left(2\pi\sigma^2\right)^{1/2}} + O\left((g\sigma/T_0)^2\right) \qquad (n=1) \ .$$

In two dimensions one has

$$\rho = \left[1 + \frac{g\sigma}{3T_0}\left(\frac{x^3}{\sigma^3} - 4\frac{x}{\sigma} + \frac{xy^2}{\sigma^3}\right)\right]\frac{e^{-\frac{x^2+y^2}{2\sigma^2}}}{2\pi\sigma^2} + O\left((g\sigma/T_0)^2\right) \qquad (n=2) \ .$$

Notice that in two or more dimensions the flux *does not vanish* in the quasistatic limit, i.e. the stationary solution is a non-equilibrium one.

In all dimensions the probability density of being in contact with the thermostat at temperature $\hat{T}$ is

$$\hat{p}(\hat{T}) = \left\langle \delta(\hat{T} - T)\right\rangle = \int d\boldsymbol{x}\, \delta\left(\hat{T} - T_0 - gx\right)\rho =$$
$$= \frac{1}{(2\pi g^2\sigma^2)^{1/2}}\left[1 + \frac{g\sigma}{3T_0}\left(\frac{(\hat{T}-T_0)^3}{g^3\sigma^3} - 3\frac{\hat{T}-T_0}{g\sigma}\right)\right] e^{-\frac{(\hat{T}-T_0)^2}{2g^2\sigma^2}} \ . \tag{S12}$$

In one dimension, the average heat release rate to the thermostat $\hat{T}$ is

$$\hat{p}(\hat{T})\dot{q}(\hat{T}) = \int dx\, \delta\left(\hat{T} - T_0 - gx\right)\left[g\frac{\partial}{\partial x}\left(\frac{1}{2\gamma}T\rho\right) - (kx+g)\,J - \frac{\partial}{\partial x}(TJ) - \frac{1}{2}\dot{T}_0\rho\right]$$

with

$$J = -\frac{T}{\gamma}\frac{\partial\rho}{\partial x} - \frac{1}{\gamma}(kx+g)\,\rho = \left[\frac{x}{\sigma} + \frac{1}{3}\frac{g\sigma}{T_0}\left(\left(\frac{x}{\sigma}\right)^4 - 3\left(\frac{x}{\sigma}\right)^2\right)\right]\dot{\sigma}\rho_0 + \dots$$

Inserting and expanding up to first order in $g\sigma/T_0$ one has

$$\hat{p}(\hat{T})\dot{q}(\hat{T}) = \int dx\, \delta\left(\hat{T} - T_0 - gx\right)\Bigg\{\rho_0\left[-T_0\left(\frac{\dot{\sigma}}{\sigma} + \frac{\dot{T}_0}{2T_0}\right) + \gamma\dot{\sigma}^2\left(\frac{x}{\sigma}\right)^2\right] +$$

$$+\rho_0\left(\frac{g\sigma}{T_0}\right)\left[\frac{x}{\sigma}\left(-\frac{\dot{\sigma}}{\sigma}T_0 + \frac{1}{2}\dot{T}_0 - \underbrace{\frac{1}{2}\frac{T_0^2}{\gamma\sigma^2}}_{anom}\right) - \left(\frac{x}{\sigma}\right)^3\left(-k\dot{\sigma}\sigma + \frac{4}{3}T_0\frac{\dot{\sigma}}{\sigma} + \frac{\dot{T}_0}{6}\right) + \frac{1}{3}\left(\frac{x}{\sigma}\right)^5\gamma\dot{\sigma}^2\right] + \Bigg\}\dots$$

Notice that for $g=0$ integrating over $x$ gives the usual definition of the rate of heat release to the (only) thermostat $\hat{T} = T_0$.

It follows that

$$\dot{q}(\hat{T}) = -T_0\frac{\dot{\sigma}}{\sigma} - \frac{1}{2}\dot{T}_0 + \gamma\dot{\sigma}^2\left(\frac{\hat{T}-T_0}{g\sigma}\right)^2 - \left(\frac{g\sigma}{T_0}\right)\left(2\frac{\dot{\sigma}T_0}{\sigma} + \frac{1}{2}\frac{T_0^2}{\gamma\sigma^2}\right)\left(\frac{\hat{T}-T_0}{g\sigma}\right) + O\left(\left(\frac{g\sigma}{T_0}\right)^2\right) \ . \tag{S13}$$

The heat is absorbed from thermostat $\hat{T}$ whenever $\dot{q}(\hat{T}) < 0$, i.e. when the equation $\dot{q} = 0$ has two real roots and the temperature is comprised in this interval.

In the quasi-equilibrium limit where all transformations take a time $\tau \gg \gamma/k \equiv \tau_r$ the prefactors of the quadratic form above scale as

$$-T_0\frac{\dot\sigma}{\sigma} - \frac{1}{2}\dot T_0 \sim \left(\frac{\gamma}{k\tau}\right)\frac{T_0 k}{\gamma}$$

$$\gamma\dot\sigma^2 \sim \gamma\frac{(T_0/k)}{\tau^2} \sim \left(\frac{\gamma}{k\tau}\right)^2\frac{T_0 k}{\gamma}$$

$$2\frac{\dot\sigma T_0}{\sigma} \sim \left(\frac{\gamma}{k\tau}\right)\frac{T_0 k}{\gamma}$$

$$\frac{1}{2}\frac{T_0^2}{\gamma\sigma^2} \sim \frac{T_0 k}{\gamma}\ .$$

As a first approximation, notice that in the quasi-equilibrium limit

$$2\frac{\dot\sigma T_0}{\sigma} \ll \frac{1}{2}\frac{T_0^2}{\gamma\sigma^2}$$

so that the linear term can be approximated as $-\left(\frac{g\sigma}{T_0}\right)\frac{T_0^2}{2\gamma\sigma^2}\left(\frac{\hat T - T_0}{g\sigma}\right)$. Comparing the remaining three terms it is useful to isolate two regimes, depending on whether $(\gamma/(k\tau))^2 \ll g\sigma/T_0$ (*i. e.* whether the linear term is dominant compared to the quadratic one) or the opposite. This introduces a timescale

$$\tau_* = \frac{\gamma}{k}\left(\frac{(T_0 k)^{1/2}}{g}\right)^{1/2}$$

which, defining the standard deviation of the equilibrium distribution $L = \sqrt{\frac{T}{k}}$, can be written as:

$$\tau_* = \left(\tau_r\frac{L\gamma}{g}\right)^{1/2} \tag{S14}$$

which, upon reintroduction of Boltzmann constant, coincides with the second term of equation (8) in the main text.

*Slow cycles:* for $\tau \gg \tau_*$ one has

$$\dot q(\hat T) \simeq -T_0\frac{\dot\sigma}{\sigma} - \frac{1}{2}\dot T_0 - \left(\frac{g\sigma}{T_0}\right)\left(\frac{1}{2}\frac{T_0^2}{\gamma\sigma^2}\right)\left(\frac{\hat T - T_0}{g\sigma}\right)$$

so that heat is absorbed when $\hat T > T_*$ where

$$\frac{T_* - T_0}{g\sigma} = -2\frac{\gamma}{g}\left(\dot\sigma + \frac{1}{2}\frac{\sigma\dot T_0}{T_0}\right)\ .$$

The rate of heat absorption is

$$\dot Q_{abs} = -\int_{T_*}^{\infty} d\hat T\, \hat p(\hat T)\dot q(\hat T)$$

with

$$\hat p(\hat T)\dot q(\hat T) = \frac{\exp\left[-(\hat T - T_0)^2/(2g^2\sigma^2)\right]}{(2\pi g^2\sigma^2)^{1/2}}\left[-T_0\left(\frac{\dot\sigma}{\sigma} + \frac{\dot T_0}{2T_0}\right) + \left(\frac{g\sigma}{T_0}\right)\left(\frac{\hat T - T_0}{g\sigma}\right)\underbrace{\left(-\frac{1}{2}\frac{T_0^2}{\gamma\sigma^2}\right)}_{anom}\right]\ .$$

Notice that in this regime the "adiabatic" transformation ($\frac{T_0^2}{k}$ = constant) implies that the only exchanged heat is due to the anomalous term.

It is possible to identify two distinct subranges in this regime, depending on the ratio of the two small parameters $g\sigma/T_0$ and $\gamma/(k\tau)$. For very long cycling times, in the limit

$$\frac{g\sigma}{T_0} \gg \frac{\gamma}{k\tau} \qquad \text{i.e.} \qquad \tau \gg \tilde{\tau} \gg \tau_*$$

with

$$\tilde{\tau} = \frac{\gamma}{k}\frac{(kT_0)^{1/2}}{g} = \frac{\gamma L}{g} \tag{S15}$$

one has

$$\left|\frac{\gamma}{g}\left(\dot{\sigma} + \frac{1}{2}\frac{\sigma\dot{T}_0}{T_0}\right)\right| \sim \frac{\gamma T_0^{1/2}}{g k^{1/2}\tau} \ll 1$$

which gives $T_* \simeq T_0$ and the heat release/absorption dominated by the anomalous contribution

$$\hat{p}(\hat{T})\dot{q}(\hat{T}) \simeq -\left(\frac{k(\hat{T}-T_0)}{2\gamma}\right)\frac{\exp\left[-(\hat{T}-T_0)^2/(2g^2T_0/k)\right]}{(2\pi g^2 T_0/k)^{1/2}}$$

where the quasi-equilibrium variance is $\sigma^2 \simeq T_0/k$. The rate of heat absorption is

$$\dot{Q}_{abs} = \frac{g}{2\gamma}\left(\frac{T_0 k}{2\pi}\right)^{1/2} . \tag{S16}$$

Conversely, if

$$\frac{g\sigma}{T_0} \ll \frac{\gamma}{k\tau} \qquad \text{i.e.} \qquad \tau_* \ll \tau \ll \tilde{\tau}$$

then

$$\left|\frac{\gamma}{g}\left(\dot{\sigma} + \frac{1}{2}\frac{\sigma\dot{T}_0}{T_0}\right)\right| \sim \frac{\gamma T_0^{1/2}}{g k^{1/2}\tau} \gg 1$$

and, depending on the sign of

$$-\left(\dot{\sigma} + \frac{1}{2}\frac{\sigma\dot{T}_0}{T_0}\right) = -\frac{1}{2\sigma T_0}\frac{d}{dt}\left(\sigma^2 T_0\right) \simeq -\frac{k^{1/2}}{T_0^{3/2}}\frac{d}{dt}\left(\frac{T_0^2}{k}\right)$$

heat is absorbed (if $\frac{d}{dt}\left(\frac{T_0^2}{k}\right) > 0$) or released (if $\frac{d}{dt}\left(\frac{T_0^2}{k}\right) < 0$) at any thermostat. During adiabatic transformations (when $\frac{d}{dt}\left(\frac{T_0^2}{k}\right)$ is identically zero) heat is absorbed or released according to the sign of the anomalous term that, albeit small, is not exactly zero.

*Intermediate cycles:* when $\gamma/k \ll \tau \ll \tau_*$ the rate of heat release is

$$\dot{q}(\hat{T}) \simeq -T_0\frac{\dot{\sigma}}{\sigma} - \frac{1}{2}\dot{T}_0 + \gamma\dot{\sigma}^2\left(\frac{\hat{T}-T_0}{g\sigma}\right)^2 .$$

During an adiabatic transformation heat is always released. During isothermal expansions heat is absorbed in the range

$$\left(\frac{T-T_0}{g\sigma}\right)^2 \leq \frac{T_0}{\gamma\sigma\dot{\sigma}} \simeq \frac{2T_0}{\gamma\frac{d}{dt}\left(\frac{T_0}{k}\right)} \sim \left(\frac{\gamma}{k\tau}\right)^{-1} \gg 1$$

implying that the heat is absorbed everywhere with exponential accuracy.

During isothermal compression the heat is always released. Therefore, we conclude that in this range the overdamped approximation with the appropriate definition of heat (considering individual thermostats) should give the correct efficiency.

*Asymptotics for efficiency*

We finally provide the asymptotic values for work and absorbed heat in the aforementioned regimes. The work is asymptotically equal to

$$W^{\infty}_{extr} = \frac{1}{2}\left(T_h - T_c\right)\log\left(\frac{k_{max}}{k_{min}}\right)$$

and is not affected by the gradient. However, the absorbed heat depends on it through the anomalous term. One has

$$Q^{\infty}_{abs} = \begin{cases} \frac{1}{2}T_h \log\left(\frac{k_{max}}{k_{min}}\right) & \tau \ll \tau_* \\ \frac{1}{2}T_h \log\left(\frac{k_{max}}{k_{min}}\right) + \frac{g}{2\gamma(2\pi)^{1/2}}\int_{adiab}\left(T_0 k\right)^{1/2} dt = \frac{1}{2}T_h \log\left(\frac{k_{max}}{k_{min}}\right) + \frac{g\tau_2\left(k_{max}^{1/2}+k_{min}^{1/2}\right)}{5\gamma T_h(T_h-T_c)(2\pi)^{1/2}}\left(T_h^{5/2} - T_c^{5/2}\right) & \tau_* \ll \tau \ll \tilde{\tau} \\ \frac{g}{2\gamma(2\pi)^{1/2}}\oint\left(T_0 k\right)^{1/2} dt = \frac{g\tau_2\left(k_{max}^{1/2}+k_{min}^{1/2}\right)}{5\gamma T_h(T_h-T_c)(2\pi)^{1/2}}\left(T_h^{5/2} - T_c^{5/2}\right) + \frac{g\tau_1\left(T_h^{3/2}+T_c^{3/2}\right)}{3\gamma T_h(k_{max}-k_{min})(2\pi)^{1/2}}\left(k_{max}^{3/2} - k_{min}^{3/2}\right) & \tau \gg \tilde{\tau} \end{cases}$$

These expressions are used to draw the asymptotes in Figure 2 of the main text, right panel.


[1] K. Sekimoto. *Stochastic energetics.* Lect. Notes Phys. 799. Springer, Berlin Heidelberg (2010).
[2] R. Chetrite and K. Gawędzki. Fluctuation relations for diffusion processes. *Commun. Math. Phys.* 282, 469518 (2008).
[3] A. Celani, S. and Bo, R. Eichhorn and E. Aurell. Anomalous thermodynamics at the micro-scale. *Physical Review Letters (in press), arXiv:1206.1742* (2012).
